# Supplementary material for: Heterogeneity for the Win: One-Shot Federated Clustering
Source: arXiv:2103.00697 source file (2021-10-05)
Supplement: Supplementary file 1 [file 08-appendixB.tex]

\section{Relaxed In-active edges}

\subsection{Preliminaries}

We now analyse the setting where we relax the strict inactive separation
requirement. That is, we allow a small fraction of points from inactive cluster
pairs to reside on each device. First, we state the following lemma, which will
be useful when controlling the error after the first step of our
algorithm\gs{what is the first step? which algorithm? it would be good to
reference a defined algorithm from the main the text}.

\begin{lemma}[Lemma 9 from
  \cite{mcsherry2001spectral}]\label{lemma:cost_ktod}\gs{Is $A$ also rank k, or
  just $C$?}
  Let $\matA$ and $\matC$ be $n\times d$ matrices, with $\rank(\matC) = k$. Let
  $\hat \matA$ be the projection of rows of $\matA$ onto the subspace spanned
  by its top $k$ singular vectors.  Then we have,
  \[
    \fbs{\hat \matA -\matC}^2 \le 8k \ops{\matA-\matC}^2.
  \]
\end{lemma}
\begin{proof} Since $\rank(\hat \matA-\matC) \le 2k$, we have,
  \[
    \fbs{\hat \matA-\matC}^2 \le 2k\ops{\hat \matA -\matC}^2 
      \le 2k\left(\ops{\hat \matA - \matA} + \ops{\matA -\matC}\right)^2
      \le 8k \ops{\matA -\matC}^2,
  \] where the last inequality follows from noting that $\ops{\matA-\hat \matA}^2 =
  \min_{\rank(\mathbf{X})=k}\ops{\matA-\mathbf{X}}^2 \le \ops{\matA-\matC}^2 $.
\end{proof}

Now we introduce the notion of \emph{large} and \emph{small} clusters.

\begin{definition}[Large and small cluster subsets] Let $m_0, m_1 > 1$ be such
  that $m_0\ll m_1.$ Let $T^z_r$ be the subset of points of cluster $T_r$ on
  device $z$. We refer to $T^z_r$ as a large subset if $\abs{T^z_r} \ge
  \frac{1}{m_0}\abs{T_r}$.  Similarly, $T^z_s$ is referred to as a small subset
  if $\abs{T^z_s} \le \frac{1}{m_1}\abs{T_s}$.\tododon{Replace $1/m_0, 1/m_1$
  by $\eps_0, \eps_1$}
\end{definition}

Intuitively, large clusters can be thought off as subsets of some target
cluster with sufficiently large number of points. Loosely speaking, cluster
means of such subsets usually are not too far away from the target cluster's
mean. Similarly, \emph{small} clusters are subsets that only contain a few
points. \gs{Is the idea that every cluster subset will either be small or
large? Do we allow clusters in between these sizes?}

Recall that by our definition, cluster pairs $r$ and $s$ form an relaxed
inactive cluster pair if, no device has `large' subsets of both clusters. That
is, w.l.g if $\abs{T^z_r} \ge \frac{1}{m_0}\abs{T_r}$ then $\abs{T^z_s} \le
\frac{1}{m_1}\abs{T_s}$. We now analyze how the presence of a few inactive
subsets affects the clustering step on each device.

Without loss of generality, let ${T^z}_{1}, {T^z}_{2}, \dots, {T^z}_{k^{'}}$ be
large subsets of $T_1, T_2, T_{k^{'}}$ on device $z$. Let $P_{1}, P_{2},
P_{\eta}$ be subsets from the remaining clustering, $T_{k^{'}+1}, \dots, T_{k}$
which forms an inactive pair with at least one of $T_1, \dots, T_{k^{'}}$. That
is, if $P_1 \subset T_{r}$ (say), then a) $r\not\in \set{1, 2, \dots, k'}$ and
b) there exists an $s \in \set{1, 2, \dots, k'}$ such that $(r, s)$ form an
inactive pair. Finally, we restrict our attention to the case where inactive
pairs are close to each other. That is, we ignore the less interesting case
where inactive pairs are far apart.\gs{Do you eventually come back to this
case? Why are you ignoring it--just to characterize things in the worst case?}
Thus we assume that for all inactive cluster pairs $(r, s)$, we have $10\lambda
\le \ltwos{\mu(T_r) - \mu(T_s)} \le c_1 \lambda$ for some sufficiently large
$c_0$.

In order to simplify notation, let $\rho =  \left(1 + \frac{\eta m_0
n_{\max}}{m_1 n_{\min}k'} + \frac{\eta c_1^2c_\lambda^2}{m_1}\right)$ and note
that $\rho \ge 1$ since all the terms are positive constants.  For the
remainder of this section, we redefine $\Delta_r$ as:
\begin{align}
    \Delta_r = k'\frac{{\ops{\matA-\matC}}}{\sqrt{n_r}}
\end{align}
With this definition, we have the following center separation lemma\gs{note:
  'lemma', 'theorem', etc should be uncapitalized unless you're referring to it
  formally with a number.  Examples: Use ``The lemma below \dots" OR ``The
  center separation lemma, below, " vs. ``Lemma 6, below, \dots" The JMLR style
guide is a good reference to check out:
https://www.jmlr.org/format/format.html}. Recall that we use the shorthand
$\mu_r$ to denote $\mu(T_r)$ and $\mu^z_r$ to denote $\mu(T^z_r)$. We also use
$n_r := \abs{T_r}$ and $n^z_r := \abs{T^z_r}$. \tododon{Be consistent with how
you define things.}

\begin{lemma}\label{lemma:centersep2} Let $(T_r, T_s)$ be cluster pairs such
  that, $\ltwo{\mu_r - \mu_s} \ge 2c\sqrt{m_0\rho}(\Delta_{r} + \Delta_s).$ Let
  $T^z_r \subseteq T_r$ and $T^z_s \subseteq T_s$ be large subsets on device
  $z$. Then,
  \begin{align*}
    \ltwo{\mu^z_r - \mu^z_s} \ge c\sqrt{m_0\rho}(\Delta_r + \Delta_s)
  \end{align*}
\end{lemma}
\begin{proof} 
  Using the triangle inequality, we have 
  \begin{align*}
    \ltwos{\mu^z_r - \mu^z_s}
      &\ge\ltwos{\mu_r - \mu_s}-\ltwo{\mu^z_r-\mu_r}-\ltwo{\mu_s-\mu^z_s}
      \ge_{(a)} 2c\sqrt{m_0\rho}(\Delta_r + \Delta_s) -
      \frac{\ops{\matA-\matC}}{\sqrt{n^z_r}}-\frac{\ops{\matA-\matC}}{\sqrt{n^z_s}}\\
      &\ge 2c\sqrt{m_0\rho}\left( k' \frac{\ops{\matA-\matC}}{\sqrt{n_r}} +  k'
      \frac{\ops{\matA-\matC}}{\sqrt{n_s}}\right) -
      \frac{\ops{\matA-\matC}}{\sqrt{n^z_r}}-\frac{\ops{\matA-\matC}}{\sqrt{n^z_s}}\\
      &\ge \left(2-\frac{1}{c \sqrt{\rho} k'}\sqrt{\frac{n_r}{n^z_r m_0}}
      \right)c\sqrt{m_0\rho} k'
      \frac{\ops{\matA-\matC}}{\sqrt{n_r}}
      + \left(2-\frac{1}{c \sqrt{\rho} k'}\sqrt{\frac{n_s}{n^z_s m_0}}
      \right)c\sqrt{m_0\rho} k'
      \frac{\ops{\matA-\matC}}{\sqrt{n_s}}\\
      &\ge_{(b)} c\sqrt{m_0\rho} k'
      \frac{\ops{\matA-\matC}}{\sqrt{n_r}}
      + c\sqrt{m_0\rho} k'
      \frac{\ops{\matA-\matC}}{\sqrt{n_s}} 
      \ge c\sqrt{m_0\rho}(\Delta_r + \Delta_s).
  \end{align*} Here inequality (a) follows from
  Lemma~\ref{lemma:meanshift} and for (b) note that $\frac{1}{c\sqrt{\rho} k'}
  \le 1$ and $n^z_r \ge \frac{1}{m_0} n_r$. Therefore, $\frac{1}{c \sqrt{\rho}
    k'}\sqrt{\frac{n_r}{n^z_r m_0}} \le 1$. Similarly, $\frac{1}{c \sqrt{\rho}
  k'}\sqrt{\frac{n_s}{n^z_s m_0}} \le 1$.
\end{proof}
\tododon{The extra $\sqrt{m_0}$ is or the lack of it here in this version of
the assumption is bothersome}

We now split the data matrix $\matA^z$ on device $z$ to certain sub matrices to
make the analysis easier.  As we did in Lemma~\ref{lemma:normchange}, lets
collect the data points indexed by $T_1^z, T_2^z, \dots, T_{k'}^z$ in a
$n^z\times d$ matrix $\matA^z_l$ and their corresponding centers in
$\matC^z_l$\tododon{Might want to explain this depending on how much
explanation is there is section A}. Further, collect points indexed by $P_{1},
P_{2},\dots P_{\eta}$ in $\matA^z_p$.  We now construct a matrix $\matC^z_p$ of
the same dimensions as $\matA^z_p$ as follows: let the $i$-th row of $\matA^z_p$ be
from some (small) cluster $P_r \subset T_r$.  Then there must exist some $s \in
{1, \dots, k'}$ such that $(r, s)$ forms an inactive pair.  Uniquely denote
such an $s$ by $g(r)$ and set $(\matC^z_p)_i = \mu{(T^z_{g(r)})}$.  That is, we
assign all points in $P_r$ to the mean of a large cluster $s$, where $(r, s)$
form an inactive pair.  We now bound the \kmeans cost of this assignment in the
following lemma.

\begin{lemma}\label{lemma:normchange_gen} Let $\matA^z$ be the data matrix on
  device $z$ and let $(\matA^z_l, \matC^z_l)$ and $(\matA^z_p, \matC^z_p)$ be
  defined as above.  Then,
  \begin{enumerate}[label=\alph*.]
    \item{
        \[
          \ops{\matA^z_l - \matC^z_l} \le 2\sqrt{k'}\ops{\matA - \matC}
        \]
        }
    \item{
    \begin{align*}
      \ops{\matA^z - \matC^z} 
        = \op{\begin{bmatrix}\matA^z_l\\\matA^z_p\end{bmatrix} -
        \begin{bmatrix}\matC^z_l\\\matC^z_p\end{bmatrix}}
        \le 2\sqrt{\rho k'}\ops{\matA-\matC}.
      \end{align*}
    }
  \end{enumerate}
\end{lemma}
\begin{proof} 
  Let $\tilde \matC^z_l, \tilde \matC^z_p$ be the matrix that contain the
  target cluster means of each point in $\matA_l^z, \matA^p_z$. That is, if the
  $i$-th row of $\matA^z_l$ belongs to $T_r$ say, then the $i$-th row of
  $\tilde\matC^z_l$ contains $\mu(T_r)$. Now note that,
  \begin{align*}
    \ops{\tilde \matC^z_l - \matC^z_l}^2 
      &=\sum_{j=1}^{k'}\abs{T^z_j}\Big(\big(\mu(T^z_j) -\mu(T_j)\big)\cdot
      u\Big)^2
      \le \sum_{j=1}^{k'}\abs{T^z_j}\ltwo{\mu(T^z_j) -\mu(T_j)}^2
      \le_{(a)} k'\op{\matA-\matC}^2.
  \end{align*}
  Here for inequality $(a)$ we invoke Lemma~\ref{lemma:meanshift}.  Also note
  that $\ops{\matA^z_l-\tilde{\matC}^z_l} \le \ops{\matA-\matC}$ since the
  matrix $(\matA^z_l - \tilde{\matC}^z_l)$ comprises of rows that are a subset
  of the rows of $(\matA - \matC)$. Thus, we have
  \begin{align*}
    \ops{\matA^z_l - \matC^z_l} 
      &\le \ops{\matA^z_l-\tilde{\matC}^z_l} + \ops{\tilde{\matC}^z_l-\matC^z_l}
    \le (1+ \sqrt{k'})\ops{\matA-\matC} 
    \le 2\sqrt{k'}\ops{\matA-\matC}.
  \end{align*} Here in for the last inequality, we used $1+\sqrt{k'} \le
  2\sqrt{k'}$ for $k' \ge 1$. This completes the proof for part (a). 

  For the next part, note that
  \begin{align*}
    \op{\begin{bmatrix}\matA^z_l\\\matA^z_p\end{bmatrix} -
      \begin{bmatrix}\matC^z_l\\\matC^z_p\end{bmatrix}}
      &\le \op{\begin{bmatrix}\matA^z_l\\\matA^z_p\end{bmatrix} -
        \begin{bmatrix}\tilde \matC^z_l\\\tilde \matC^z_p\end{bmatrix}} + 
         \op{\begin{bmatrix}\matC^z_l\\\matC^z_p\end{bmatrix} -
          \begin{bmatrix}\tilde \matC^z_l\\\tilde \matC^z_p\end{bmatrix}}\\
      &\le_{(a)} \op{\matA-\matC} + 
         \op{\begin{bmatrix}\matC^z_l\\\matC^z_p\end{bmatrix} -
          \begin{bmatrix}\tilde \matC^z_l\\ \tilde \matC^z_p
        \end{bmatrix}}\numberthis\label{eq:temp01_lemma6}.
  \end{align*} Here inequality (a) follows from noting that the matrix from
  the first term is just a subset of rows of matrix $({\matA-\matC})$. Now we need to
  bound the second term. Let $u$ be any unit vector along the top singular
  direction of this matrix. Recall that $g(j)$ denotes the target set to which
  all points of $P_j$ are assigned. Then, $\mu^z_{g(j)} := \mu(T^z_{g(j)})$, denote
  the mean to which all points in $P_j$ are assigned. Then we have,
  \begin{align*}
    \op{\begin{bmatrix}\matC^z_l\\\matC^z_p\end{bmatrix} -
        \begin{bmatrix}\tilde \matC^z_l\\\tilde \matC^z_p\end{bmatrix}}^2
      &= \sum_{j=1}^{k'}\abs{T^z_j}
      \left((\mu(T^z_j) - \mu(T_j))\cdot u\right)^2 +
      \sum_{j=1}^{\eta}\abs{P_j}\left((\mu^z_{g(j)} - \mu(T_j))\cdot
      u\right)^2\\
      &\le \sum_{j=1}^{k'}\abs{T^z_j}\ltwos{\mu(T^z_j) - \mu(T_j)}^2 + 
      \sum_{j=1}^{\eta}\abs{P_j}\ltwos{\mu^z_{g(j)} - \mu(T_j)}^2\\
      &\le k'\ops{\matA-\matC}^2 + 
      \sum_{j=1}^{\eta}\abs{P_j}\ltwos{\mu^z_{g(j)} - \mu(T_j)}^2,
      \numberthis\label{eq:temp02_lemma6}
  \end{align*} where we applied Lemma~\ref{lemma:meanshift} in the last
  inequality. We now bound the second term,
  \tododon{$c_\lambda = 5\sqrt{m_0}$}
  \begin{align*}
    \sum_{j=1}^{\eta}\abs{P_j}\ltwos{\mu^z_{g(j)} - \mu(T_j)}^2
      &\le \sum_{j=1}^{\eta}\abs{P_j}\ltwos{\mu^z_{g(j)} - \mu_{g(j)}}^2
      + \sum_{j=1}^{\eta}\abs{P_j}\ltwos{\mu_{g(j)} - \mu(T_j)}^2\\
      &\le_{(a)} \sum_{j=1}^{\eta}\abs{P_j}\frac{\ops{\matA-\matC}^2}{{n^z_{g(j)}}}
      + \sum_{j=1}^{\eta}\abs{P_j}c_1^2c_\lambda^2k'\frac{\ops{\matA-\matC}^2}{n_j}\\
      &\le \ops{\matA-\matC}^2\sum_{j=1}^{\eta}\frac{\abs{P_j}}{{n^z_{g(j)}}}
      + c_1^2c_\lambda^2k'{\ops{\matA-\matC}^2}\sum_{j=1}^{\eta}\frac{\abs{P_j}}{n_j}\\
      &\le_{(b)} \ops{\matA-\matC}^2\sum_{j=1}^{\eta}\frac{\abs{P_j}}{{n^z_{g(j)}}}
      + c_1^2c_\lambda^2k'{\ops{\matA-\matC}^2}\frac{\eta}{m_1}
  \end{align*} Here for
      inequality (a), for the first term we used Lemma~\ref{lemma:meanshift}
      and for the second term, we used our assumption that for inactive cluster
      pairs $(r, s)$, ${10 \lambda \le \ltwos{\mu(T_r) - \mu(T_s)} \le c_1
        \lambda}$\tododon{ix assumption; should be $\lambda_r$ and what not}.
        For inequality (b), we used the fact that $\abs{P_j} \le
        \frac{1}{m_1}n_j$. Now recall that $n_{\max} = \max_j \abs{T_j}$ and
        $n_{\min} = \min_j \abs{{T_j}}$. We thus can write, 
  \begin{align*}
    \sum_{j=1}^{\eta}\abs{P_j}\ltwos{\mu^z_{g(j)} - \mu(T_j)}^2
      &\le
      \ops{\matA-\matC}^2\sum_{j=1}^{\eta}
        \frac{\frac{1}{m_1}n_{\max}}{\frac{1}{m_0}n_{\min}}
      + c_1^2c_\lambda^2k'{\ops{\matA-\matC}^2}\frac{\eta}{m_1}
      \le \left(\frac{m_0n_{\max}}{n_{\min}}
      + c_1^2c_\lambda^2k'\right){\ops{\matA-\matC}^2}\frac{\eta}{m_1}
  \end{align*} 
  Plugging this into~\eqref{eq:temp02_lemma6} we get,
  \begin{align*}
    \op{\begin{bmatrix}\matC^z_l\\\matC^z_p\end{bmatrix} -
      \begin{bmatrix}\tilde \matC^z_l\\\tilde \matC^z_p\end{bmatrix}}^2 
      &\le k'\ops{\matA-\matC}^2 + \left(\frac{m_0 n_{\max}}{n_{\min}}
      + c_1^2c_\lambda^2k'\right){\ops{\matA-\matC}^2}\frac{\eta}{m_1}\\
      &\le \left(1 + \frac{\eta m_0 n_{\max}}{k' m_1 n_{\min}}
      + \frac{\eta c_1^2c_\lambda^2}{m_1}\right)k'{\ops{\matA-\matC}^2}
      \le \rho k' \ops{\matA-\matC}^2.
  \end{align*} We use this in~\eqref{eq:temp01_lemma6}, to conclude our proof
  \begin{align*}
    \op{\begin{bmatrix}\matA^z_l\\\matA^z_p\end{bmatrix} -
      \begin{bmatrix}\matC^z_l\\\matC^z_p\end{bmatrix}}
      &\le (1 + \sqrt{\rho k'})\ops{\matA-\matC}  
      \le 2\sqrt{\rho k'}\ops{\matA-\matC}.
  \end{align*} 
\end{proof}

\begin{lemma}\label{lemma:costub} Let $\matA^z$ be the data matrix on device $z$ and let $(\matA^z_l, \matC^z_l)$ and $(\matA^z_p, \matC^z_p)$ be defined as above. Let $\hat
  \matA^z_p$ denote the projection of $\matA^z_p$ onto the top $k'$ singular direction
  of $\matA^z$.  Then,
  \[
    \fbs{\hat \matA^z_l-  \matC^z_l}^2 + \fbs{\hat \matA^z_p - \matC^z_p}^2 \le
    32n_r \rho\Delta_r ^2.
  \]
\end{lemma}
\begin{proof} Consider the following,
  \begin{align*}
    \fbs{\hat \matA^z_l-\matC^z_l}^2 + \fbs{\hat \matA^z_p - \matC^z_p}^2 
      &= \fb{\begin{bmatrix}\hat \matA^z_l\\\hat \matA^z_p\end{bmatrix} 
        - \begin{bmatrix}\matC^z_l\\\matC^z_p\end{bmatrix}}^2.
    \end{align*}
    Note that $\rank(\matC^z_l) = k'$ and rows of $\matC^z_p$ are a subset of rows of
    $\matC^z_l$. Therefore, 
    \[
      \rank\left(\begin{bmatrix}
          \matC^z_l\\\matC^z_p
      \end{bmatrix}\right) = k'.
    \] Applying Lemma~\ref{lemma:cost_ktod}, and then
    Lemma~\ref{lemma:normchange_gen}, we complete the proof.
    \begin{align*}
    \fbs{\hat \matA^z_l-\matC^z_l}^2 + \fbs{\hat \matA^z_p - \matC^z_p}^2 
      &\le 8k'\op{\begin{bmatrix}\matA^z_l\\\matA^z_p\end{bmatrix} 
        - \begin{bmatrix}\matC^z_l\\\matC^z_p\end{bmatrix}}^2
      \le 32\rho k'^2\ops{\matA-\matC}^2\\
      &\le 32 \rho \left( k'\frac{\ops{\matA-\matC}}{\sqrt{n_r}}\right)^2n_r
      \le 32n_r \rho\Delta_r^2.
  \end{align*} 
\end{proof}

Now we bound the `initialization' error on each device using the following
Lemma.
\begin{lemma}\label{lemma:init_error} Let $T^z_r$ be the subset of points of
  cluster $T_r$ on device $z$. Assume $T^z_r$ is a large cluster and let
  $\mu_r^z = \mu(T_r^z)$. Then after step 1 of~\algoA, for every $r$, there
  exists a center $\nu_s$ such that 
  \[
    \norm{\mu^z_r - \nu_s} \le 20\sqrt{\rho \frac{n_r}{n^z_r}}\Delta_r
      \le 20 \sqrt{m_0\rho}\Delta_r
  \]
\end{lemma}
\begin{proof} Let us use $\nu_{d(i)}$ to denote the center returned by the
  approximation algorithm, that is closest to $\hat A^z_i, i \in T^z_r$.
  Further let $R = \min_{j}\ltwo{\mu^z_r - \nu_j}$. Now consider the
  contribution of points in $T^z_r$ to the total \kmeans-cost.
  \begin{align*}
    \sum_{i \in T^z_r}\ltwos{\hat{A}^z_i - \nu_{d(i)}}^2
      &= \sum_{i \in T^z_r}\ltwos{(\mu^z_r - \nu_{d(i)}) - (\mu^z_r - \hat A
      ^z_i)}^2\\
      &>_{(a)} \sum_{i \in T^z_r}\frac{\ltwos{\mu^z_r - \nu_{d(i)}}^2}{2} - 
        \sum_{i \in T'_r}\ltwos{\hat{A}^z_i - \mu^z_r}^2\\
      &\ge_{(b)} \frac{n^z_r}{2}R^2 - \fbs{\hat{\matA}^z_l-\matC^z_l}^2
      \ge_{(c)} \frac{n^z_r}{2}R^2 - 8k'\ops{\matA^z_l - \matC^z_l}^2.
  \end{align*} Here for (a) we used the fact that $(a-b)^2 \ge \frac{1}{2}a^2 -
  b^2$. For (b) we note that $\sum_{i\in T^z_r}\ltwos{\hat{A}^z_i - \mu^z_r}^2 \le
  \fbs{\hat{\matA}^z_l - \matC^z_l}$ and finally for (c) we apply
  Lemma~\ref{lemma:cost_ktod}.

  Let $\phi^*$ be the optimum \kmeans-cost. Since we used a 10-approximation
  algorithm in step 1 of \algoA, the \kmeans-cost of the assignment after step
  1 is at most $10\phi^*$. Note that,
  \[
    \phi^* \le \fbs{\matA^z_l-\matC^z_l}^2 + \fbs{\matA^z_p - \matC^z_p}^2.
  \] Thus, the contribution of points indexed by $T^z_r$ must satisfy,
  \begin{align*}
    \frac{n^z_r}{2}R^2 - 8k'\ops{\matA^z_l-\matC^z_l}^2 
      &\le \sum_{i \in T^z_r}\ltwos{\hat{A}^z_i - \nu_{d(i)}}^2 
      \le 10(\fbs{\matA^z_l-\matC^z_l}^2 + \fbs{\matA^z_p - \matC^z_p}^2)
  \end{align*} Applying Lemma~\ref{lemma:costub} and solving,
  \begin{align*}
    \frac{n^z_r}{2}R^2 - 8k'\ops{\matA^z_l-\matC^z_l}^2 
      &\le 320n_r\rho\Delta_r^2\\
    \frac{n^z_r}{2}R^2  
      &\le 320n_r\rho\Delta_r^2+ 8k'\ops{\matA^z_l-\matC^z_l}^2
      \le_{(a)} 320n_r\rho\Delta_r^2+ 8k'\left(2\sqrt{\rho k'}
      \ops{\matA-\matC}\right)^2\\
      &\le 400n_r\rho\Delta_r^2\\
    R &\le 20\sqrt{\rho\frac{n_r}{n^z_r}}\Delta_r 
    \le_{(b)} 20\sqrt{m_0\rho}\Delta_r.
  \end{align*}
  Here inequality (a) follows from Lemma~\ref{lemma:normchange_gen},
  $\ops{\matA^z_l - \matC^z_l} \le 2\sqrt{k'\rho}\ops{\matA-\matC}$. For (b) we
  used $n^z_r \ge \frac{1}{m_0}n_r$.
\end{proof}

\subsection{Stage-1 bound}

{
  \newcommand{\aA}{\mathcal{A}}
  \newcommand{\sm}{S_r^{-}}
  \newcommand{\omegao}{\omega_{\text{out}}}
  \newcommand{\omegai}{\omega_{\text{in}}}
  \begin{lemma}Denote $\aA_r = \set{u \mid (u, r) \text{ are inactive
    pairs}}$. Denote $\sm = S_r \setminus \left(\cup_{u \in \aA_r}^{\eta}P_u\right)$.
    Then for every $r$, we have 
    \[
      \ltwos{\mu(\sm) - \mu^z_r} 
      \le {5\sqrt{m_0k'}}\frac{\ops{\matA-\matC}}{\sqrt{n_r}}
      \le \frac{5\sqrt{m_0}}{\rho \sqrt{k'}}\Delta_r.
    \]
\end{lemma}
\begin{proof} Let $\omegao$ be such that $\sm$ contains all but
  $\omegao$ fraction of points of $T^z_r$. That is, $\abs{\sm \cap T^z_r} =
  (1-\omegao) n^z_r$. Similarly for both $s \ne r$ and $u \not\in \aA$ define
  $\omegai(s)$ such that $\abs{\sm \cap T^z_s} = \omegai(s)n^z_r$ and $\abs{\sm
  \cap P^z_u} = \omegai(u)n^z_r$. Then, we have,
  \begin{align*}
    \ltwos{\mu(\sm) - \mu^z_r} 
    &= \ltwo{\frac{(1-\omegao)n^z_r\cdot \mu(\sm \cap T^z_r) 
        + \sum_{s\ne r}\omegai(s)n^z_r\cdot\mu(\sm\cap T^z_s)}
        {(1 - \omegao + \sum_{s\ne r}\omegai(s))n^z_r} - \mu^z_r}\\
    &= \ltwo{\frac{(1-\omegao)n'_r\cdot (\mu(\sm \cap T'_r) - \mu'_r) + \sum_{s \ne
          r}\omegai(s)n'_r \cdot (\mu(\sm\cap T'_s) - \mu'_r)}{(1- \omegao + \sum_{s\ne
    r}\omegai(s))n'_r}}\\
    &\le \frac{(1-\omegao)n'_r\ltwos{\mu(\sm \cap T'_r) - \mu'_r} + \sum_{s \ne
        r}\omegai(s)n'_r \ltwos{\mu(\sm\cap T'_s) - \mu'_r}}{(1- \omegao + \sum_{s\ne
    r}\omegai(s))n'_r}\\
    &\le \frac{(1-\omegao)n'_r\ltwos{\mu(\sm \cap T'_r) - \mu'_r} + 
        \frac{3}{2}\sum_{s \ne r}\omegai(s)n'_r \ltwos{\mu(\sm\cap T'_s) -
          \mu'_s}}{(1- \omegao + \sum_{s\ne r}\omegai(s))n'_r}\\
    &\le \frac{1}{(1 - \omegao + \sum_{s\ne r}\omegai(s))n'_r}
    \left({\sqrt{(1-\omegao)n'_r}\ops{A'-C'} + \frac{3}{2}\sum_{s \ne
      r}\sqrt{\omegai(s)n'_r}\ops{A'-C'}}\right)\\
    &\le \left(\frac{{\sqrt{(1-\omegao)} + \frac{3}{2}\sum_{s \ne
    r}\sqrt{\omegai(s)}}} {1 - \omegao + \sum_{s\ne r}\omegai(s)}\right)
    \frac{\ops{A'-C'}}{\sqrt{n'_r}}.\numberthis\label{lemma13:temp01}
  \end{align*} \tododon{Simplify and add explanations} Now from
  Lemma~\ref{lemma:} we know that $\omegao \le \frac{1024}{c^2\rho^2}$ and
  similarly from Lemma~\ref{lemma:} we have, $\omegai(s) \le
  \left(\frac{(48\sqrt{2})^2}{c^4\rho^4k'^2}\right)$. Note that, $\omegao \le
  \frac{1}{4}$ and $\sum_{s\ne r}\omegai(s) \le
  \frac{(48\sqrt{2})^2}{c^4\rho^4k'}\le \frac{(48\sqrt{2})^2}{c^4k'} \le
  \frac{1}{4k'}$. This means that the denominator,
  \[
    1 - \omegao + \sum_{s \ne r} \omegai(s) \ge \frac{3}{4}.
  \] We can thus write \eqref{lemma13:temp01} as,
  \begin{align*}
    \ltwos{\mu(\sm) - \mu'_r} 
    &\le \frac{4}{3}\left({{\sqrt{(1-\omegao)} + \frac{3}{2}\sum_{s \ne
    r}\sqrt{\omegai(s)}}}\right)
    \frac{\ops{A'-C'}}{\sqrt{n'_r}}
    \le \frac{4}{3}\left({1 + \frac{3}{2}\sum_{s \ne
    r}\sqrt{\omegai(s)}}\right)
    \frac{\ops{A'-C'}}{\sqrt{n'_r}}\\
    &\le_{(a)} \frac{4}{3}\left({1 + \frac{3\sqrt{k'}}{2}\sqrt{\sum_{s \ne
    r}\omegai(s)}}\right) \frac{\ops{A'-C'}}{\sqrt{n'_r}}
    \le_{(b)} \frac{4}{3}\left({1 + \frac{3}{4}}\right)
    \frac{\ops{A'-C'}}{\sqrt{n'_r}}\\
    &\le \frac{7}{3}\frac{\ops{A'-C'}}{\sqrt{n'_r}}
    \le_{(c)} \frac{14\sqrt{k'}}{3}\frac{\ops{A-C}}{\sqrt{n'_r}}
    \le 5\sqrt{m_0k'}\frac{\ops{A-C}}{\sqrt{n_r}}
    \le \frac{5\sqrt{m_0}}{\rho \sqrt{k'}}\Delta_r.
  \end{align*}
\end{proof}
}
\subsection{Classification Lower Bound}\label{sec:classification_lb}

Our goal is to bound the number of points from $T^z_r$ that are not correctly
classified to $S_r$ after step 2 of~\algoA. We will argue that most points of
$T_r^z$ are in fact correctly classified into $S_r$. 

We do this in two steps. First in
Lemma~\ref{lemma:chareterize_classifications} we give a condition that a
point $A^z_i$ must satisfy to ensure $i \in S_r$. Later in
Lemma~\ref{lemma:classification_lb} we argue that most points in $T^z_r$
satisfy this condition and are thus correctly classified establishing an upper
bound on misclassification in the process.

\begin{lemma}\label{lemma:chareterize_classifications} Let $T^z_r$ be a
  large subset of $T_r$ on device $z$ and let $\mu^z_r = \mu(T^z_r)$. Let
  $A^z_i$ be some point on this device. If $\ltwos{\hat A^z_i - \mu^z_r} \le
  \frac{c\sqrt{m_0\rho}}{8}\Delta_r$, then after step 2 of \algoA, $i \in S_r$.
\end{lemma}
\begin{proof} Observe that,\tododon{We implicitly assume $v_r$ is near
  $\mu^z_r$. This needs to be specified. Moreover, should it be $v^z_r$?
  This is an countrapositive statement. There are points not
    necessarily in $T^z_r$ that satisfy the above condition. They will also be
  classified into $S_r$. The way we use lemma 11 in lemma 12 is impt.}
  \begin{align*}
    \ltwos{\hat A^z_i - v_r} 
      \le \ltwos{\hat A^z_i - \mu^z_r} + \ltwos{\mu^z_r - v_r}
      \le \left(\frac{c}{8} + 20\right)\sqrt{m_0\rho}\Delta_r 
      \le \frac{c}{4}\sqrt{m_0\rho}\Delta_r,
  \end{align*} for $c \ge 160$. On the other hand, for any $s \ne r$,
  \begin{align*}
    \ltwos{\hat A^z_i - v_s} 
      &\ge \ltwos{\mu^z_r  - \mu^z_s} - \ltwos{\hat A^z_i  - \mu^z_r} -
      \ltwos{\mu^z_s - \nu_s} 
      \ge c\sqrt{m_0\rho}(\Delta_r + \Delta_s) - 
      \frac{c\sqrt{m_0\rho}}{8}\Delta_r - 20\sqrt{m_0\rho}\Delta_s\\
      &\ge \left(c-\frac{c}{8}\right)\sqrt{m_0\rho}\Delta_r 
      + (c-20)\sqrt{m_0\rho}\Delta_s \ge \frac{7c}{8}\sqrt{m_0\rho}\Delta_r
      \ge 3\left(\frac{c}{4}\sqrt{m_0\rho}\Delta_r\right)
      \ge 3 \ltwos{\hat A^z_i - \nu_r}.
  \end{align*} Therefore, $\ltwos{\hat A^z_i - \nu_r} \le \frac{1}{3}\ltwos{\hat
  A^z_i - \nu_s}$, and thus $i \in S_r$ completing the proof.
\end{proof}

Observe that Lemma~\ref{lemma:chareterize_classifications} holds for any
$A^z_i$ regardless of which cluster it belongs to. Now let us consider $i \in
T^z_r$ on device $z$. If $i$ is such that $\ltwos{\hat A^z_i - \mu^z_r} >
\frac{c}{8}\sqrt{m_0\rho}\Delta_r$, then it is possible that $i \not\in S_r$.
Let $U_r = \set{ i \mid i \in T^z_r, \ltwos{\hat A^z_i - \mu^z_r} >
\frac{c}{8}\sqrt{\rho m_0}\Delta_r}$. The set $U_r$ indexes into the subsets of
points of $T^z_r$ that could be misclassified. We use the following lemma to
bound $\abs{U_r}$.

\begin{lemma}\label{lemma:classification_lb} Let $T_r^z$ be a large
  subset of $T_r$ on a device $z$ and let $U_r = \set{ i \mid i
  \in T^z_r, \ltwos{\hat A^z_i - \mu^z_r} > \frac{c}{8}\sqrt{m_0\rho}\Delta_r}$ and
  let $\setc{S}_r$ denote the set compliment of set $S_r$. Then, $\abs{T^z_r
  \cap \setc{S}_r} \le \abs{U_r} \le \frac{2048}{c^2\rho}n^z_r$ and
  $\abs{T^z_r \cap S_r} \ge \big(1-\frac{2048}{c^2\rho}\big)n^z_r$.
\end{lemma}
\begin{proof} Consider the contribution of points indexed by $U_r$ to the total
  \kmeans cost on this device after step-$1$.
  \begin{align}
    \sum_{i \in U} \ltwos{\hat A^z_i - \mu^z_r}^2 
      &\le \fbs{\hat \matA^z_l - \matC^z_l}^2 
      \le_{(a)} 8k'\ops{\matA^z_l-\matC^z_l}^2
      \le_{(b)}32k'^2\ops{\matA-\matC}^2\label{lemma10_01}.
  \end{align} Here we used Lemma~\ref{lemma:cost_ktod} for inequality (a) and
  Lemma~\ref{lemma:normchange_gen} for inequality (b). But for $i \in U_r$,
  $\ltwos{\hat A^z_i - \mu^z_r} > \frac{c}{8}\sqrt{m_0\rho}\Delta_r$, therefore
  \begin{align}
    \sum_{i \in U_r}\ltwos{\hat A^z_i - \mu^z_r}^2 
    \ge \abs{U_r}\frac{c^2}{64}m_0\rho\Delta_r^2\label{lemma10_02}
  \end{align} Combining, \eqref{lemma10_01} and \eqref{lemma10_02}, we get,
  \begin{align*}
    \abs{U_r} 
      &\le \frac{2048k'^2\ops{\matA-\matC}^2}{c^2 m_0\rho \Delta_r^2}
      \le \frac{2048k'^2\ops{\matA-\matC}^2n_r}{c^2 m_0 \rho k'^2\ops{\matA-\matC}^2}
    \le \frac{2048}{c^2\rho}\left(\frac{1}{m_0}n_r\right)
    \le \frac{2048}{c^2\rho}n^z_r.
  \end{align*} Consider any point $A^z_i, i \in T^z_r$ that do not belong to
  $S_r$. That is, points in $T^z_r \cap \setc{S}_r$. According to
  Lemma~\ref{lemma:chareterize_classifications}, such point must have
  $\ltwos{\hat A^z_i - \mu^z_r} > \frac{c\sqrt{m_0}\rho}{8}\Delta_r$ and thus $i
  \in U_r$. That is $T^z_r \cap \setc{S}_r \subseteq U_r$ and therefore,
  $\abs{T^z_r \cap \setc{S}_r} \le \abs{U_r} \le \frac{2048}{c^2\rho}n^z_r$.
  Now $\abs{T^z_r \cap S_r} = \abs{T^z_r} - \abs{T^z_r \cap \setc{S}_r}
  \ge\big(1-\frac{2048}{c^2\rho}\big)n^z_r$ completing the proof.
\end{proof}

\subsection{Missclassification Upper Bound}\label{sec:missclassification_ub}

Here, our goal is to bound the number of points from $T^z_s$, $s \ne r$ that
are incorrectly classified to $S_r$ after step 2 of~\algoA. We roughly follow a
similar approach to that used in establishing the classification lower bound
(Section~\ref{sec:classification_lb}). First in
Lemma~\ref{lemma:charecterize_missclassification} we give a condition that a point
$A^z_i$ for an $i \not\in T^z_r$ must satisfy to not be in $S_r$.
Later in Lemma~\ref{lemma:missclassification_ub} we argue that most points
in $T^z_s$, $s \ne r$ satisfy this condition and are thus not in $S_r$,
establishing our bound. Further, we also argue that most points from small
cluster subset $P_u$ do not belong to $S_r$, if $(u, r)$ forms an active pair.
 
\begin{lemma}\label{lemma:charecterize_missclassification} Let $\matA^z$ be the
  data matrix on device $z$. Let $T^z_r$ and $T^z_s$ be large subsets of $T_r$
  and $T_s$ on this device with $\mu^z_r = \mu(T^z_r)$ and $\mu^z_s =
  \mu(T^z_s)$. Let $\hat \mu^z_r$ and $\hat\mu^z_s$ be the projection of
  $\mu^z_r$ and $\mu^z_s$ along the top $k'$ singular directions of $\matA^z$.
  Fix $r$ and consider $i \not\in T^z_r$ such that there exists an $s (s \ne
  r)$, for which $\ltwos{\hat A^z_i - \hat \mu^z_s}< 2\ltwos{\hat A^z_i - \hat
    \mu^z_r}$, then $\ltwos{\hat A^z_i - v_s} < 3 \ltwos{\hat A^z_i - v_r}$ and
    thus $i \not \in S_r$.
\end{lemma}
\begin{proof} Since  $\ltwos{\hat A^z_i - \hat \mu^z_s}< 2\ltwos{\hat A^z_i -
  \hat \mu^z_r}$ we can upper bound $\ltwos{\hat A^z_i - \nu_s}$ as,
  \[
    \ltwos{\hat A^z_i - \nu_s} 
    \le \ltwos{\hat A^z_i - \hat\mu^z_s} + \ltwos{\hat\mu^z_s - \nu_s}
    <_{(a)} 2\ltwos{\hat A^z_i - \hat \mu^z_r} + \ltwos{\mu^z_s - \nu_s}
  \]
  Here for inequality (a), we use the fact that the vector $(\hat \mu_s^z -
  \nu_s)$ is a projection of $(\mu_s^z - \nu_s)$ and thus $\ltwos{\hat \mu_s^z
    - \nu_s} \le \ltwos{\mu_s^z - \nu_s}$. Also, for $\ltwos{\hat A^z_i -
  \nu_r}$ we have the following lower bound,
  \[
    \ltwos{\hat A^z_i - \nu_r} \
    \ge \ltwos{\hat A^z_i - \hat \mu^z_r} - \ltwos{\hat \mu^z_r - \nu_r}
    \ge \ltwos{\hat A^z_i - \hat \mu^z_r} - \ltwos{\mu^z_r - \nu_r}.
  \] We now claim that,
  \begin{align}
    3(\ltwos{\hat A^z_i - \hat \mu^z_r} - \ltwos{\mu^z_r - \nu_r})
    > 2\ltwos{\hat A^z_i - \hat \mu^z_r} + \ltwos{\mu^z_s -
    \nu_s}.\label{lemma11:temp02}
  \end{align} Assuming the claim is true, we have
  \begin{align*}
    \ltwos{\hat A^z_i - \nu_s} 
      \le  2\ltwos{\hat A^z_i - \hat \mu^z_r} + \ltwos{\mu^z_s - \nu_s}
      < 3(\ltwos{\hat A^z_i - \hat \mu^z_r} - \ltwos{\mu^z_r - \nu_r})
      \le 3\ltwos{\hat A^z_i - \nu_r},
  \end{align*} and thus, we get the required result,
    \[
        \ltwos{\hat A^z_i - \nu_s} \le 3\ltwos{\hat A^z_i - \nu_r}.
    \] 
      
  Now we prove our claim~\eqref{lemma11:temp02}, through contradiction. Assume
  the claim is false and let,
  \begin{align*}
    3(\ltwos{\hat A^z_i - \hat \mu^z_r} - \ltwos{\mu^z_r - \nu_r})
    &\le 2\ltwos{\hat A^z_i - \hat \mu^z_r} + \ltwos{\mu^z_s - \nu_s}\\
    \ltwos{\hat A^z_i - \hat \mu^z_r}
    &\le \ltwos{\mu^z_s - \nu_s} + 3\ltwos{\mu^z_r - \nu_r}
    \le 3(\ltwos{\mu^z_s - \nu_s} + \ltwos{\mu^z_r - \nu_r})\\
    &\le 60\sqrt{m_0\rho}(\Delta_r + \Delta_s)\numberthis\label{lemma11:temp01}.
  \end{align*} But since $\ltwos{\hat A^z_i - \hat \mu^z_s} < 2\ltwos{\hat
  A^z_i - \hat\mu^z_r}$, from the triangle inequality we have,
  \begin{align*}
    \ltwos{\hat \mu^z_r - \hat \mu^z_s}  - \ltwos{\hat A^z_i - \hat\mu^z_r} 
    \le 
    \ltwos{(\hat \mu^z_r - \hat \mu^z_s) + (\hat A^z_i - \hat\mu^z_r)} 
    < 2 \ltwos{\hat A^z_i - \hat \mu^z_r}.
  \end{align*} Therefore,
  \begin{align*}
    3\ltwos{\hat A^z_i - \mu^z_r} 
      &> \ltwos{\hat \mu^z_r - \hat \mu^z_s}
      = \ltwos{(\mu^z_r - \mu^z_s) + (\hat \mu^z_r -  \mu^z_r)  
        + (\mu^z_s - \hat \mu^z_s)}\\
      &\ge \ltwos{\mu^z_r - \mu^z_s} - \ltwos{\hat \mu^z_r -  \mu^z_r} 
        -\ltwos{\mu^z_s - \hat \mu^z_s}\\
      &\ge \ltwos{\mu^z_r - \mu^z_s} - (\ltwos{\hat \mu^z_r - \nu_r}+
      \ltwos{\nu_r-  \mu^z_r} )- (\ltwos{\hat \mu^z_s - \nu_s}+
      \ltwos{\nu_s-  \mu^z_s} )\\
      &\ge_{(a)} \ltwos{\mu^z_r - \mu^z_s} - 2\ltwos{\mu^z_r - \nu_r} 
      - 2\ltwos{\nu_s-  \mu^z_s}\\
      &\ge_{(b)} c\sqrt{m_0\rho}(\Delta_r + \Delta_s) 
      - 40\sqrt{m_0\rho}\Delta_r - 40\sqrt{m_0\rho}\Delta_s
      \ge ({c-40})\sqrt{m_0\rho}(\Delta_r + \Delta_s)\numberthis\label{lemma11:temp04}.
  \end{align*} Here for inequality (a), we again use the fact that the vector
  $(v_r - \hat\mu^z_r)$ is a projection of $(\nu_r - \mu^z_r)$ and thus
  $\ltwos{\nu_r - \hat\mu^z_r} \le \ltwos{\nu_r - \mu^z_r}$. For (b) we used
  Lemma \ref{lemma:init_error} and our center separation assumptions. On
  simplifying~\eqref{lemma11:temp04} for $c \ge 220$ we see that, $\ltwos{\hat
  A^z_i - \mu^z_r} > 60\sqrt{m_0\rho}(\Delta_r + \Delta_s)$, contradicting
  \eqref{lemma11:temp01} and thus completing the proof.
\end{proof}

Lemma~\ref{lemma:charecterize_missclassification} holds for any $i \not\in
T^z_r$. We consider two specific cases. First, consider an $i$ that is part of
some fixed large subset $s$, i.e. $i \in T^z_s$ $(s \ne r)$. If $\ltwos{\hat
A^z_i - \hat \mu^z_s} \ge 2 \ltwos{\hat A^z_i - \hat \mu^z_r}$ then $A^z_i$ could
potentially be misclassified into $S_r$. Secondly, consider $i$ in some small
subset $P_u$ where $(u, r)$ form an active pair and $(u, s)$ form an inactive
pair($u, r, s$ are fixed). Again, if $\ltwos{\hat A^z_i - \hat \mu^z_s} \ge 2
\ltwos{\hat A^z_i - \hat \mu^z_r}$ then $i$ could be misclassified into $S_r$.
We now proceed to upper bound both of these potential missclassifications.

\begin{figure}[h]
  \centering
  \includegraphics[width=0.75\textwidth]{img/proj01.jpg}
  \caption{caption}
  \label{fig:appendix:01}
\end{figure}

Recall that $\hat A^z_i$ is the projection of $A^z_i$ onto the top $k'$
singular directions of $A^z$. For the next lemma, we will be using projections
heavily. Lets denote with $\hat\mu^z_s$ the projection of $\mu^z_s$ onto the
same subspace. Let us also denote with $\dot{A}^z_i$ the projection of $A^z_i$
onto the line between $\hat \mu^z_r$ and $\hat \mu^z_s$. Observe that (see
Figure~\ref{fig:appendix:01}),
\[
  \ltwos{\hat A^z_i - \hat \mu^z_s}^2 
    = \ltwos{\hat A^z_i - \dot A^z_i}^2 + \ltwos{\dot A^z_i-\hat \mu^z_s}^2,
  \quad\text{and,}\quad
  \ltwos{\hat A^z_i - \hat \mu^z_r}^2 = \ltwos{\hat A^z_i - \dot A^z_i}^2 +
  \ltwos{\dot A^z_i - \hat \mu^z_r}^2.
\] This means that for points with $\ltwos{\hat A^z_i - \hat \mu^z_s} \ge 2
\ltwos{\hat A^z_i - \hat \mu^z_r}$, we also have $\ltwos{\dot A^z_i - \hat
\mu^z_s} \ge 2 \ltwos{\dot A^z_i - \hat \mu^z_r}$. Using the triangle
inequality, we get
\begin{align*}
  \ltwos{\dot A^z_i - \hat \mu^z_s} 
    &\ge 2 (\ltwos{\hat \mu^z_r - \hat \mu^z_s} - 
      \ltwos{\dot A^z_i - \hat \mu^z_s})\\
  \ltwos{\dot A^z_i  - \hat \mu^z_s} 
    &\ge \frac{2}{3}\ltwos{\hat \mu^z_r - \hat\mu^z_s}.
\end{align*} Since $\ltwos{\dot A^z_i - \hat
  \mu^z_r} \le \frac{1}{2}\ltwos{\dot{A}^z_i - \hat \mu^z_s}$,
\begin{align*}
  \ltwos{\dot A^z_i - \hat \mu^z_s} - \ltwos{\dot A^z_i - \hat \mu^z_r}
  \ge \frac{1}{2}\ltwos{\dot A^z_i - \hat \mu^z_s} 
  \ge \frac{1}{3}\ltwos{\hat \mu^z_r - \hat
  \mu^z_s}.\numberthis\label{lemma:charecterize_missclassification2}
\end{align*}We summarize this relationship in the following corollary.
\begin{corollary}\label{corollary:condition_intermediate}
  For a fixed $r$ and an $i \not\in T^z_r$, if for some $s$,
$\ltwos{\hat A^z_i - \hat \mu^z_s} \ge 2\ltwos{\hat A^z_i - \hat \mu^z_r}$ then
$ \ltwos{\dot A^z_i - \hat \mu^z_s} - \ltwos{\dot A^z_i - \hat \mu^z_r} \ge
\frac{1}{3}\ltwos{\hat \mu^z_r - \hat \mu^z_s}$.
\end{corollary}

Now fix $(r, s, u)$ and let $X_s$ be the set of such points from $T^z_s$ that
satisfies~\eqref{lemma:charecterize_missclassification2}. Thus $X_s$ contains the
points from $T^z_s$ that could be missclassified into $S_r$. Further, recall that
$P_u$ was a small subset from $T_u$ such that $(u, r)$ form an active pair and
$(u, s)$ form an inactive pair. Let $Y_u$ be the set of points from $P_u$ that
satisfy~\eqref{lemma:charecterize_missclassification2} and could possibly be
missclassified into $S_r$. We now use the following lemma to bound the size of
both $X_s$ and $Y_u$.  A variation of this lemma was originally proven
in~\cite{kumarkannan01} and later simplified
by~\cite{awasthisheffet01}. We adapt the proof from the later work for
this presentation.

\begin{lemma}\label{lemma:missclassification_ub} Fix $r, s$ and  let $\matA^z$
  be the data matrix on device $z$. Let $T^z_r$ and $T^z_s$ be large subsets of
  $T_r$ and $T_s$ on this device for some $s$.  Denote with $\mu^z_r =
  \mu(T^z_r)$ and let $\hat \mu^z_r$ be the projection of $\mu^z_r$ along the
  top $k'$ singular directions of $\matA^z$.  Additionally, let $\dot A^z_i$
  denote the projection of $A^z_i$ onto the line connecting $\hat \mu^z_r$ and
  $\hat \mu^z_s$. Let $P_u$ be any small cluster such that $(u, r)$ form an
  active pair and $(u, s)$ form an inactive pair.
  Define
  \begin{align*}
    X &= \set{i \mid i \in T^z_s, \ltwos{\dot A^z_i -
      \hat\mu^z_s} - \ltwos{\dot A^z_i - \hat \mu^z_r}\ge
    \frac{1}{3}\ltwos{\hat\mu^z_r - \hat\mu^z_s}},\\
        Y_{u} &= \set{i \mid i \in P_u, \ltwos{\dot A^z_i -
      \hat\mu^z_s} - \ltwos{\dot A^z_i - \hat \mu^z_r}\ge
      \frac{1}{3}\ltwos{\hat\mu^z_r - \hat\mu^z_s}}.
  \end{align*}
  Define $Y_u := \phi$ if no such $u$ exists. Then, $\abs{X \cup Y_u} \le
  \frac{96^2}{c^4 k'^2}\cdot n^z_r$.
\end{lemma}

Before we prove this lemma, let us build some intuition.
Lemma~\ref{lemma:charecterize_missclassification} tells us that any point $i
\in X \cup Y_u$  will be `far' from $\hat\mu^z_s$ in the projected subspace
since,
\[
  \ltwos{\dot A^z_i - \hat\mu^z_s} \ge \ltwos{\dot A^z_i - \hat \mu^z_r}
    + \frac{1}{3}\ltwos{\hat\mu^z_r - \hat\mu^z_s}.
\] We use this intuition to get a lower bound on $\ltwos{A^z_i -
  \mu^z_s}$. This will give us a lower bound on the contribution of such points
  to the total clustering cost. We  employ the Markov inequality to bound the
  number of such points that can exist without exceeding the total clustering
  cost to obtain our result.

{\newcommand{\pv}{P_{\mathcal{V}}}
  \begin{proof} Let $\mathcal{V}$ denote the subspace spanned by $\set{\mu^z_r,
    \mu^z_s, \hat\mu^z_r, \hat\mu^z_s}$ and let $\pv(A^z_i)$ denote the
    projection of $A^z_i$ onto this subspace. We now prove a few small facts
    that will be useful in the proof.
    
    Firstly, since $\pv(A^z_i)$ lies on a subspace containing the line between
    $\hat\mu^z_r$ and $\hat\mu^z_s$, projecting $A^z_i$ onto this line is the
    same as projecting $\pv(A^z_i)$ onto this line. That is, $\dot A^z_i = \dot
    \pv(A^z_i)$. Now, for $i \in X
    \cup Y_u$,
  \begin{align*}
  \ltwos{\dot A^z_i - \hat\mu^z_s} -\ltwos{\dot A^z_i - \hat \mu^z_r}
    \ge \frac{1}{3}\ltwos{\hat\mu^z_r - \hat\mu^z_s}
    \iff
    \ltwos{\dot\pv(A^z_i) - \hat\mu^z_s} -\ltwos{\dot\pv(A^z_i) - \hat \mu^z_r}
    \ge \frac{1}{3}\ltwos{\hat\mu^z_r - \hat\mu^z_s}.
    \label{lemma14:temp01}\numberthis
  \end{align*} Secondly, we use the fact that $\ltwos{\mu^z_r - \hat\mu^z_r}$
  is small, a fact originally proven by~\cite{achlioptasmcsherry01}. Let
  $u_r$ be the indicator vector of points in $T^z_r$.
  \begin{align*}
    \ltwos{\mu^z_r - \hat\mu^z_r} 
    &= \frac{1}{n^z_r}\ltwos{(\matA^z_l - \hat \matA^z_l)\tr\cdot u_r}
    \le \frac{1}{n^z_r}\ops{\matA^z_l - \hat \matA^z_l}\ltwos{u_r}
    \le_{(a)} \frac{1}{\sqrt{n^z_r}}\ops{\matA^z_l-\matC^z_l}.
    \numberthis\label{lemma14:temp03}
  \end{align*} Here for (a), we first used the fact that $\ops{\matA^z_l -
  \hat\matA^z_l} = \min_{\rank(\mathbf{Z}) = k'} \ops{\matA^z_l-\mathbf{Z}} \le
  \ops{\matA^z_l-\matC^z_l}$ and then the fact that $\ltwos{u} = \sqrt{n'_r}$.

  Finally, using the triangle inequality with~\eqref{lemma14:temp01} we note that,
  \begin{align*}
    \frac{1}{3}\ltwos{\hat\mu^z_r - \hat\mu^z_s}
    &\le \Big(\ltwos{\pv(A^z_i) - \hat\mu^z_s} + \ltwos{\dot\pv(A^z_i) -
    \pv(A^z_i)}\Big)
    -\Big(\ltwos{\pv(A^z_i) - \hat \mu^z_r} - \ltwos{\dot\pv(A^z_i)-\pv(A^z_i)}\Big)\\
    &\le \ltwos{\pv(A^z_i) - \hat\mu^z_s} -\ltwos{\pv(A^z_i) - \hat \mu^z_r}
    \numberthis\label{lemma14:temp02}
  \end{align*} This essentially tells us that $ \ltwos{\pv(A^z_i) - \mu^z_s}
  \ge\ltwos{\pv(A^z_i) - \hat\mu^z_r}$. 

  Now we proceed to our main arguments. Due to the Pythagoras theorem, for both
  $\hat\mu^z_s$ and $\hat\mu^z_s$ we have,
  $\ltwos{\pv(A^z_i) - \hat\mu^z_s}^2 = \ltwos{\dot\pv(A^z_i) - \hat\mu^z_s}^2
  + \ltwos{\dot\pv(A^z_i)- \pv(A^z_i)}^2 $. Thus, 
  \begin{align*}
    \ltwos{\pv(A^z_i) - \hat\mu^z_s}^2 -\ltwos{\pv(A^z_i) - \hat \mu^z_r}^2
    &\ge (\ltwos{\dot\pv(A^z_i) - \hat\mu^z_s} -\ltwos{\dot\pv(A^z_i) - \hat \mu^z_r})
     (\ltwos{\dot\pv(A^z_i) - \hat\mu^z_s} +\ltwos{\dot\pv(A^z_i) - \hat \mu^z_r})\\
    &\ge \frac{1}{3}\ltwos{\hat\mu^z_r - \hat\mu^z_s}
    (\ltwos{\dot\pv(A^z_i) - \hat\mu^z_s} +\ltwos{\dot\pv(A^z_i) - \hat \mu^z_r})\\
    &\ge \frac{1}{3}\ltwos{\hat\mu^z_r - \hat\mu^z_s}^2
    \numberthis\label{lemma12:lb}
  \end{align*} We have now established a lower bound on 
  $\ltwos{\pv(A^z_i) - \hat\mu^z_s}^2 -\ltwos{\pv(A^z_i) - \hat
  \mu^z_r}^2$. We now establish an upper bound on the same quantity in terms of
  $\ltwos{\pv(A^z_i)-\mu_s^z}$. Using the triangle inequality, we have
    \begin{align*}
      \ltwos{\pv(A^z_i) - \hat\mu^z_s} 
      &\le \ltwos{\pv(A^z_i) - \mu^z_s} + \ltwos{\hat\mu^z_s - \mu^z_s}
      \le_{(a)} \ltwos{\pv(A^z_i) - \mu^z_s}
        +\frac{1}{\sqrt{n^z_s}}\ops{\matA^z_l-\matC^z_l}\\
      &\le \ltwos{\pv(A^z_i) - \mu^z_s} +
      \left(\frac{1}{\sqrt{n^z_s}} +
      \frac{1}{\sqrt{n^z_r}}\right)\ops{\matA^z_l-\matC^z_l}.
      \numberthis\label{lemma12:temp02}
    \end{align*} Here we used~\eqref{lemma14:temp01} for inequality (a). Similarly,
    \begin{align*}
      \ltwos{\pv(A^z_i) - \hat\mu^z_r}
      \ge \ltwos{\pv(A^z_i) - \mu^z_s} - \left(\frac{1}{\sqrt{n^z_s}} +
       \frac{1}{\sqrt{n^z_r}}\right)\ops{\matA^z-\matC^z}.
       \numberthis\label{lemma12:temp03}
     \end{align*} For notational convenience, let $\beta =
     \left(\frac{1}{\sqrt{n^z_s}} +
     \frac{1}{\sqrt{n^z_r}}\right)\ops{\matA^z_l-\matC^z_l}$.
       Combining~\eqref{lemma12:temp02} and~\eqref{lemma12:temp03} we have,
     \begin{align*}
      \ltwos{\pv(A^z_i) - \hat\mu^z_s}^2 - \ltwos{\pv(A^z_i) - \hat\mu^z_r}^2  
      &\le \left(\ltwos{\pv(A^z_i) - \mu^z_s} + \beta\right)^2 
        - \left(\ltwos{\pv(A^z_i) - \mu^z_r} - \beta\right)^2 \\
      &\le_{(a)} \left(\ltwos{\pv(A^z_i) - \mu^z_s} + \beta\right)^2 
        - \left(\ltwos{\pv(A^z_i) - \mu^z_s} - \beta\right)^2 \\
      &\le 4\beta\ltwos{\pv(A^z_i) - \mu^z_s}.\numberthis\label{lemma12:ub}
     \end{align*} Here for (a) we used~\eqref{lemma14:temp02}. On combining our
     lower bound from~\eqref{lemma12:lb} and our upper bound
     from~\eqref{lemma12:ub}, we get
     \begin{align*}
      \frac{1}{3}\ltwos{\hat\mu^z_r - \hat\mu^z_s}^2 
      \le \ltwos{\pv(A^z_i) - \hat\mu^z_s}^2 - \ltwos{\pv(A^z_i)-\hat\mu^z_r}^2
      &\le 4\beta\ltwos{\pv(A^z_i) - \mu^z_s}.
     \end{align*} Stated differently, we have
     \begin{align*}
       \ltwos{\pv(A^z_i) - \mu^z_s}
       \ge \frac{1}{12\beta}\ltwos{\hat\mu^z_r -
       \hat\mu^z_s}^2.\numberthis\label{lemma12:temp05}
     \end{align*} From Lemma~\ref{lemma:centersep2} we know that
     $\ltwos{\mu^z_r - \mu^z_s} \ge c\sqrt{m_0\rho}(\Delta_r + \Delta_s)$ and from
     Lemma~\ref{lemma:normchange_gen} we know that
     $\frac{\ops{\matA-\matC}}{\ops{\matA^z_l-\matC^z_l}} \ge
     \frac{1}{2\sqrt{k'}}$. Further, from our assumption on large clusters we
     know that $n^z_r \ge \frac{1}{{m_0}}n_r$, which implies
     $\frac{1}{\sqrt{n^z_r}} \le \sqrt{\frac{m_0}{n_r}}$. We use these facts to
     simplify~\eqref{lemma12:temp05},
     \begin{align*}
       \ltwos{\pv(A^z_i) - \mu^z_s} 
       &\ge \frac{c^2{m_0\rho}}{12\beta}(\Delta_r + \Delta_s)^2
       \ge\frac{c^2\rho k'^2}{12\beta}\left(\sqrt{\frac{{m_0}}{{n_r}}} + 
     \sqrt{\frac{{m_0}}{{n_s}}}\right)^2\ops{\matA-\matC}^2\\
       &\ge\frac{c^2\rho k'^2\sqrt{m_0}}{12\beta}\left({\frac{{1}}{\sqrt{n_r}}} + 
       {\frac{1}{\sqrt{n_s}}}\right)\left({\frac{{1}}{\sqrt{n^z_r}}} + 
       {\frac{1}{\sqrt{n^z_s}}}\right)\ops{\matA-\matC}^2\\
       &\ge\frac{c^2\rho
         k'^2\sqrt{m_0}}{24\sqrt{k'}}\left({\frac{{1}}{\sqrt{n_r}}} + 
       {\frac{1}{\sqrt{n_s}}}\right)\ops{\matA-\matC}
       \ge\frac{c^2\rho k'^2\sqrt{m_0}}{24\sqrt{k'}\sqrt{n_r}}
       \ops{\matA-\matC}.
     \end{align*}

     Now using this we bound the $\abs{X \cup Y_u}$. Observer that,
     \begin{align*}
       \abs{X\cup Y_u}\left(\frac{c^2\rho
       k'^2\sqrt{m_0}}{24\sqrt{k'}\sqrt{n_r}}\right)^2\ops{\matA-\matC}^2
       &\le \sum_{i \in X_s} \ltwos{\pv(A^z_i) - \mu^z_s}^2
       + \sum_{i \in P_u} \ltwos{\pv(A^z_i) - \mu^z_s}^2\\
       &\le\fbs{\pv(\matA^z_l-\matC^z_l)}^2+\fbs{\pv(\matA^z_p-\matC^z_p)}^2
       \le_{(a)} 4\ops{\pv(\matA^z-\matC^z)}^2\\
       &\le 4\ops{\matA^z-\matC^z}^2 \le 16k'\rho^2\ops{\matA-\matC}^2.
     \end{align*} Here for (a) we note that $\pv(\matA^z-\matC^z)$ is the
     projection onto a $4$ dimensional subspace $\mathcal{V}$. Thus the rank of
     $\pv(\matA^z-\matC^z)$ is at most $4$. On simplifying, we get $\abs{X_s
     \cup Y_u} \le \frac{96^2}{c^4k'^2}\cdot n^z_r$ as required,
     completing the proof.
\end{proof}
}

\begin{corollary}\label{corollary:missclassification_ub} Fix $r$ and  let
  $\matA^z$ be the data matrix on device $z$. Let $T^z_r$ and $T^z_s$ be large
  subsets of $T_r$ and $T_s$ on this device. Let $P_u$ be a small subset of
  $T_u$. Then, after step 2 of~\algoA,
  \begin{enumerate}[label=\alph*.]
    \item{for every large subset $T^z_s$, for $s \ne r$
         \[
           \abs{T_s^z \cap S_r} 
           \le \abs{X} 
           \le \frac{96^2}{c^4 k'^2}\cdot n^z_r
         \]
      }
    \item{for a small subset $P_u$ that forms an active pair with $r$ and an
        inactive pair with some $s$,
         \[
           \abs{P_u \cap S_r} 
           \le \abs{Y_u} 
           \le \frac{96^2}{c^4 k'^2}\cdot n^z_r.
         \]
      }
  \end{enumerate}
\end{corollary}
\begin{proof}From
  Lemma~\ref{lemma:charecterize_missclassification} we know that for any $i \in
  S_r$ and for all $s \ne r, \ltwos{\hat A^z_i - \hat \mu^z_s} \ge 2
  \ltwos{\hat A^z_i - \hat \mu^z_r}$. Specifically, any $i \in T^z_s \cap S_r$
  also satisfies this condition. Also $s, r, i$ also satisfies the requirements
  for Corollary~\ref{corollary:condition_intermediate}. Thus by definition $i
  \in X$ and $ T^z_s \cap S_r \subseteq X$. Applying
  Lemma~\ref{lemma:missclassification_ub} completes the proof of the first
  part.  The proof for the second part follows similarly by noting that $P_u
  \cap S_r \subseteq Y_u$.
\end{proof}
